# Supplementary material for: Resilient Coverage: Exploring the Local-to-Global Trade-off
Source: arXiv:1910.01917 source file (2020-04-15)
Supplement: Supplementary file 1 [file appendix.tex]

\section*{Appendix}
\paragraph{\textbf{Distributed clique cover}} 
We execute our distributed non-overlap clique cover algorithm in three communication rounds and one computation round as shown in Algorithm~\ref{alg:DNCCA}.
\begin{enumerate}
\item \textit{1st communication}:  each robot $i$ finds its neighbors within its communication range as $\mathcal{N}_i$ (Alg.~\ref{alg:DNCCA}, line~\ref{line:ncc_find_nei}). It then stores its neighbors and itself in the set $\mathcal{N}^+_i$ (Alg.~\ref{alg:DNCCA}, line~\ref{line:ncc_set_i_nei}). 
\item \textit{2nd communication}: each robot $i$ shares the set $\mathcal{N}^+_i$ with all of its neighbors (Alg.~\ref{alg:DNCCA}, line~\ref{line:ncc_share_nei}). After the sharing, it receives all $\mathcal{N}^+_j, j\in\mathcal{N}_i$ from its neighbors (Alg.~\ref{alg:DNCCA}, line~\ref{line:ncc_rece_nei}). We arbitrarily order these sets as $\mathcal{N}^+_{j1}, \cdots,  \mathcal{N}^+_{j|\mathcal{N}_i|}$ for the convenience of expression. It then stores the set $\mathcal{N}^+_i$ and all $\mathcal{N}^+_j$ from its neighbors in a super set $\mathcal{N}^{+}=\{\mathcal{N}^+_i, \mathcal{N}^+_{j1}, \cdots,  \mathcal{N}^+_{j|\mathcal{N}_i|}\}$ (Alg.~\ref{alg:DNCCA}, line~\ref{line:ncc_store_nei_nei}). \item \textit{computation}: Given the super set $\mathcal{N}^{+}$, each robot $i$ first finds all of its maximal cliques by computing the intersections among $m$ subsets in $\mathcal{N}^{+}$ from $m= |\mathcal{N}^{+}|$ to $m=2$ in a loop (Alg.~\ref{alg:DNCCA}, lines~\ref{line:ncc_m_for_1}-\ref{line:ncc_m_for_end}). With a slight abuse of notation, we denote $|\mathcal{N}^{+}|$ as the number of the subsets in $\mathcal{N}^{+}$. In the loop, for each value of $m$, there are $\binom{|\mathcal{N}^{+}|}{m}$ possible intersections (Alg.~\ref{alg:DNCCA}, line~\ref{line:ncc_all_combs}). The robot $i$ stores all the intersections whose cardinality equals to $m$ in a super set $\mathcal{C}^{i}$ (Alg.~\ref{alg:DNCCA}, lines~\ref{line:ncc_com_for_1}-\ref{line:ncc_com_for_end}). Once the super set $\mathcal{C}^{i}$ is non-empty, the robot $i$ sets its maximal clique set $\mathcal{C}^{i*}$ as $\mathcal{C}^{i}$ (Alg.~\ref{alg:DNCCA}, lines~\ref{line:ncc_non_empty}-\ref{line:ncc_maximal_cliques}). The loop with descending order of $m$ terminates (Alg.~\ref{alg:DNCCA}, line~\ref{line:ncc_mfor_break}). 
% Again, for the convenience of expression, we write the intersections in $\mathcal{C}^{i*}$ in an arbitrary order as $\{\mathcal{C}^{i*}_{1},\cdots,\mathcal{C}^{i*}_{j}, \cdots \mathcal{C}^{i*}_{|\mathcal{C}^{i*}|}\}$. 
After finding all maximal cliques, the robot $i$ decides its unique maximal clique.
If there is only one intersection (subset) in $\mathcal{C}^{i}$, the robot $i$ sets its unique maximal clique $\mathcal{C}^{iu}$ as $\mathcal{C}^{i*}$ (Alg.~\ref{alg:DNCCA}, lines~\ref{line:ncc_one_subset}-\ref{line:ncc_set_one_unique}). Otherwise, it computes the neighbors for all the intersections (subsets) in $\mathcal{C}^{i*}$. Here, we compute the neighbors of a set of robots as the union of the neighbors from all the individual robots within this set.  It then picks the intersection which has fewest neighbors as its unique maximal clique $\mathcal{C}^{iu}$ (Alg.~\ref{alg:DNCCA}, line~\ref{line:ncc_pick_one_unique}). 
\item \textit{3rd communication}: each robot $i$ shares its unique maximal clique with all of its neighbors (Alg.~\ref{alg:DNCCA}, line~\ref{line:ncc_share_unique}). 
\end{enumerate}

The robots belong to the same unique clique formulate a unique clique of the graph $\mathcal{G}$. A unique clique can have one robot only. After all unique cliques are identified, the non-overlapping clique cover is achieved on the graph $\mathcal{G}$. Since each robot finds its unique clique based on the local information only, Algorithm~\ref{alg:DNCCA} is a feasible or sub-optimal (not global optimal) solution for covering the graph with the minimum number of non-overlapping cliques. However, the key point in Algorithm~\ref{alg:DNCCA} is the way that each robot decides its unique maximal clique when it has two or more maximal cliques. Since the robot picks the maximal clique with fewest neighbors, it increases the potential for other maximal cliques to formulate other larger cliques, which leads to a higher chance of generating fewer and larger non-overlapping cliques.
\begin{algorithm}[t]
\caption{Distributed Non-overlap Clique Cover}
\begin{algorithmic}[1]
\REQUIRE
\begin{itemize}
    \item set of robots $\mathcal{R}$
    \item positions the robots 
    \item communication range $r_c$
\end{itemize}
\ENSURE  Non-overlapping clique cover on graph $\mathcal{G}$
\STATE \textbf{for} each robot $i$ \textbf{do}
\STATE \hspace{2mm} finds its neighbor set $\mathcal{N}_i$ within $r_c$ \label{line:ncc_find_nei}
\STATE \hspace{2mm}  sets $\mathcal{N}_i^{+} = \{i, \mathcal{N}_i\}$
\label{line:ncc_set_i_nei}
\STATE \hspace{2mm} shares $\mathcal{N}_i^{+}$ with its neighbors
\label{line:ncc_share_nei}
\STATE \hspace{2mm} receives all $\mathcal{N}_j^{+}, j\in\mathcal{N}_i$ 
\label{line:ncc_rece_nei}
\STATE \hspace{2mm}  stores $\mathcal{N}_i^{+}$ and  all $\mathcal{N}_j^{+}(s)$ in \\
\hspace{2mm} $\mathcal{N}^{+}=\{\mathcal{N}^+_i, \mathcal{N}^+_{j1}, \cdots,  \mathcal{N}^+_{j|\mathcal{N}_i|}\}$
\label{line:ncc_store_nei_nei}
\STATE \hspace{2mm} $\mathcal{C}^{i} \leftarrow \emptyset$;
\STATE \hspace{2mm} \textbf{for} $m = |\mathcal{N}^{+}| : 2$ 
\label{line:ncc_m_for_1}
\STATE \hspace{4mm} compute all combinations of $m$ subsets from \\
\hspace{4mm} $\mathcal{N}^{+}$ as 
$\binom{\mathcal{N}^{+}}{m}$
\label{line:ncc_all_combs}
\STATE \hspace{4mm} \textbf{for} each combination in $\binom{\mathcal{N}^{+}}{m}$ $\textbf{do}$
\label{line:ncc_com_for_1}
\STATE \hspace{6mm} computes its intersection, $\mathcal{C}_{\text{intersect}}$
\STATE \hspace{6mm} \textbf{if} $|\mathcal{C}_{\text{intersect}}| = m$ \textbf{do}
\STATE \hspace{8mm} puts $\mathcal{C}_{\text{intersect}}$ in $\mathcal{C}^{i}$
\STATE \hspace{6mm} \textbf{end if}
\STATE \hspace{4mm} \textbf{end for}
\label{line:ncc_com_for_end}
\STATE \hspace{4mm} \textbf{if} $\mathcal{C}^{i}$ is not empty
\label{line:ncc_non_empty}
\STATE \hspace{6mm} sets its maximal clique set $\mathcal{C}^{i*} = \mathcal{C}^{i}$
\label{line:ncc_maximal_cliques}
\STATE \hspace{6mm} breaks the \textbf{for loop} of  $m$
\label{line:ncc_mfor_break}
\STATE \hspace{4mm} \textbf{end if} 
\STATE \hspace{2mm} \textbf{end for}
\label{line:ncc_m_for_end}
\STATE \hspace{2mm} \textbf{if} $\mathcal{C}^{i*}$ only has one subset \textbf{do}
\label{line:ncc_one_subset}
\STATE \hspace{4mm} sets its unique maximal clique as $\mathcal{C}^{iu} = \mathcal{C}^{i*}$
\label{line:ncc_set_one_unique}
\STATE \hspace{2mm} \textbf{else}
\STATE \hspace{4mm} chooses the subset of $\mathcal{C}^{i*}$ that has fewest neighbors
\label{line:ncc_pick_one_unique}
\STATE \hspace{2mm} \textbf{end if}
\STATE \hspace{2mm} shares its unique clique with all of its neighbors
\label{line:ncc_share_unique}
\STATE \textbf{end for}
\end{algorithmic}
\label{alg:DNCCA}
\end{algorithm}
%%%%%%%%%%%%%%%%%%%%%%%%%%%%%%%%%%

\paragraph{\textbf{Proof for Theorem~\ref{thm:DRA}}}
We first provide the following notations for the convenience of the proof.  

Denote the optimal selection as $\mathcal{S}^{\star}$ with $|\mathcal{S}^{\star}|\leq N$. $\mathcal{S}^{\star} = \bigcup_{k=1}^{\mathcal{K}}\mathcal{S}^{\star}_k$  where $\mathcal{S}^{\star}_k, ~k\in\{1,\cdots, \mathcal{K}\}$ is the set selected by the optimal in each clique $\mathcal{C}_k$,  and $|\mathcal{S}^{\star}_k| \leq n_k$. Denote the worst-case attack on the optimal set $\mathcal{S}^{\star}$ with respect to the whole network $\mathcal{G}$ as $\mathcal{A}^{\star}(\mathcal{S}^{\star}|\mathcal{G})$ with $|\mathcal{A}^{\star}(\mathcal{S}^{\star}|\mathcal{G})|\leq \alpha$.  Similarly, denote the set selected by the Algorithm   as $\mathcal{S}$ with $|\mathcal{S}|\leq N$. $\mathcal{S} = \bigcup_{k=1}^{\mathcal{K}}\mathcal{S}_k$  where $\mathcal{S}_k, ~k\in\{1,\cdots, \mathcal{K}\}$ is the set selected in each clique $\mathcal{C}_k$ with $|\mathcal{S}_k| \leq n_k$. Denote the worst-case attack on the chosen set $\mathcal{S}$ with respect to the overall graph as $\mathcal{A}^{\star}(\mathcal{S}|\mathcal{G})$ with $|\mathcal{A}^{\star}(\mathcal{S}|\mathcal{G})|\leq \alpha$. 

\textbf{Proof of approximation ratio.} In Algorithm~\ref{alg:DRA}, all cliques of robots in parallel select out strategy set $\mathcal{S}$. In fact, these cliques together rank out the \emph{central $\alpha$ largest set}.  That is because, the oblivious strategies from all cliques are the union set of all \emph{local $\alpha$ largest sets} or \emph{local clique-size largest sets}, which is a superset of the \emph{central $\alpha$ largest set}. But this \emph{central $\alpha$ largest set} is unknown to each clique. We partition the strategy set $\mathcal{S}$ from Algorithm~\ref{alg:DRA} into $\mathcal{S}_1^{\alpha}$ and $\mathcal{S}_2$. $\mathcal{S}_1^{\alpha}$ denotes the \emph{central $\alpha$ largest set} and $\mathcal{S}_2 =\mathcal{S}\setminus \mathcal{S}_1^{\alpha}$, corresponding to the strategies on the subgraph $\mathcal{G}_{2}$ (Fig.~\ref{fig:fd_graph_G}-(b)). 

We prove the approximation ratio of Algorithm~\ref{alg:DRA} by proving the following three inequalities.
\begin{align}
&\frac{f(\mathcal{S}\setminus \mathcal{A}^\star(\mathcal{S}))}{f^\star}\geq\frac{1-\nu_{f}(\mathcal{I})}{2} f(\mathcal{S}^{\star}\setminus \mathcal{A}^{\star}(\mathcal{S}^{\star}|\mathcal{G})), \label{ineq:thm1_appx_ratio1} \\ 
& \text{If}~\mathcal{K}(\mathcal{G}) = 1: \frac{f(\mathcal{S}^{}\setminus \mathcal{A}^\star(\mathcal{S}^{}))}{f^\star}\geq\nonumber\\
& \frac{1}{2} \max[\frac{1}{\alpha+1}, \frac{1}{N-\alpha}]  f(\mathcal{S}^{\star}\setminus \mathcal{A}^{\star}(\mathcal{S}^{\star}|\mathcal{G})), \label{ineq:thm1_appx_ratio2}\\
& \text{If}~\mathcal{K}(\mathcal{G}) \geq 2: \frac{f(\mathcal{S}^{}\setminus \mathcal{A}^\star(\mathcal{S}^{}))}{f^\star}\geq\nonumber\\
& \max[\frac{1}{\alpha+1}, \frac{1}{N-\alpha}] \frac{1}{\mathcal{K}(\mathcal{G}_2)}\frac{1}{\omega(\mathcal{G}_2)} f(\mathcal{S}^{\star}\setminus \mathcal{A}^{\star}(\mathcal{S}^{\star}|\mathcal{G})).\label{ineq:thm1_appx_ratio3}
\end{align}
Note that the number of cliques in subgraph $\mathcal{G}_2$, $\mathcal{K}(\mathcal{G}_2)\geq 1$, since $\alpha < N$. We start with the proof of the ineq.~\ref{ineq:thm1_appx_ratio1} by using the property of the curvature $\nu_f(\mathcal{I})$.  \begin{align}
&f(\mathcal{S}^{}\setminus \mathcal{A}^{\star}(\mathcal{S}^{}|\mathcal{G}))\nonumber \\ &\geq (1-\nu_{f}(\mathcal{I})) \sum_{a\in \mathcal{S}_2^{}|\mathcal{G}_2}f(a) \label{ineq:thm1_curv_ratio1}\\
&\geq (1-\nu_{f}(\mathcal{I})) \sum_{a\in \mathcal{S}^{g}_{2}|\mathcal{G}_2}f(a) \label{ineq:thm1_curv_ratio2}\\
&\geq (1-\nu_{f}(\mathcal{I})) f(\mathcal{S}^{g}_{2}|\mathcal{G}_2) \label{ineq:thm1_curv_ratio3}\\
& \geq \frac{1-\nu_{f}(\mathcal{I})}{2} 
%1+\nu_{f}(\mathcal{I})
f(\mathcal{S}_{2}^{\star}|\mathcal{G}_2) \label{ineq:thm1_curv_ratio4}\\
& \geq \frac{1-\nu_{f}(\mathcal{I})}{2} f(\mathcal{S}^{\star}\setminus \mathcal{A}^{\star}(\mathcal{S}^{\star}|\mathcal{G}))~\label{ineq:thm1_curv_ratio5}
\end{align}
where eqs.~\ref{ineq:thm1_curv_ratio1} -   \ref{ineq:thm1_curv_ratio5} hold for the following reasons. Ineq.~\ref{ineq:thm1_curv_ratio1} follows from~\cite[Lemma 2 and the proof of Theorem 1]{tzoumas2018resilient}. It is based on the property of the curvature and the fact that every element in $\mathcal{S}_1^{\alpha}$ is larger than every element in $\mathcal{S}_{2}^{}|\mathcal{G}_2$. In ineq.~\ref{ineq:thm1_curv_ratio2}, $\mathcal{S}_{2}^{g} |\mathcal{G}_2$ denotes the strategy set selected by the greedy algorithm with centralized communication on the subgraph $\mathcal{G}_2$. While $\mathcal{S}_{2}^{} |\mathcal{G}_2$ is the strategy set selected by the resilient algorithm in parallel (Alg.~\ref{alg:DRA}) on the subgraph $\mathcal{G}_2$. We know the greedy algorithm with centralized communication avoids more redundancy than the distributed resilient algorithm (Alg.~\ref{alg:DRA}) does. Thus, the value $f(a), a \in \mathcal{S}_{2}^{}$ is always larger or equal to the value $f(a'), a'\in \mathcal{S}_{2}^{g}$ where $a$ and $a'$ are the strategies from the same robot. Then, ineq.~\ref{ineq:thm1_curv_ratio2} holds. Ineq.~\ref{ineq:thm1_curv_ratio3}  holds from the submodularity of the function $f$.  Ineq.~\ref{ineq:thm1_curv_ratio4}  holds from the property of the greedy algorithm~\cite[Theorem 2.3]{conforti1984submodular} and $\mathcal{S}_{2}^{\star} |\mathcal{G}_2$ denotes the optimal strategy set on the subgraph $\mathcal{G}_2$. Finally, ineq.~\ref{ineq:thm1_curv_ratio5}  holds from ~\cite[Lemma 2]{orlin2018robust}. 

When the communication graph $\mathcal{G}$ has one clique only, Algorithm~\ref{alg:DRA} is exactly the centralized resilient submodular maximization algorithm from~\cite[Algorithm 1]{zhou2019resilient}, and thus ineq.~\ref{ineq:thm1_appx_ratio2} holds accordingly from~\cite[Theorem 1]{zhou2019resilient}. 

Finally, we prove the third ineq.~\ref{ineq:thm1_appx_ratio3} as follows. 
\begin{align}
&f(\mathcal{S}^{}\setminus \mathcal{A}^{\star}(\mathcal{S}^{}|\mathcal{G}))\nonumber\\ &\geq \gamma f(\mathcal{S}_2|\mathcal{G}_2)\label{ineq:thm1_na_ratio1}\\
& \geq \gamma \frac{1}{\mathcal{K}(\mathcal{G}_2)} \sum_{k=1}^{\mathcal{K}(\mathcal{G}_2)} f(\mathcal{S}_{2,k}^{}|\mathcal{C}_k(\mathcal{G}_2))\label{ineq:thm1_na_ratio2}\\
& \geq \gamma \frac{1}{\mathcal{K}(\mathcal{G}_2)} \sum_{k=1}^{\mathcal{K}(\mathcal{G}_2)} h_{k}^{} f(\mathcal{S}_{2,k}^{\star}|\mathcal{C}(\mathcal{G}_2))\label{ineq:thm1_na_ratio3}\\
& \geq \gamma \frac{1}{\mathcal{K}(\mathcal{G}_2)}\min_{k} h_{k}^{} \sum_{k=1}^{\mathcal{K}(\mathcal{G}_2)} f(\mathcal{S}_{2,k}^{\star}|\mathcal{C}_k(\mathcal{G}_2))\label{ineq:thm1_na_ratio4}\\
& \geq \gamma \frac{1}{\mathcal{K}(\mathcal{G}_2)}\frac{1}{\omega(\mathcal{G}_2)} f(\mathcal{S}_{2}^{\star}|\mathcal{G}_2)\label{ineq:thm1_na_ratio5}\\
& \geq \gamma \frac{1}{\mathcal{K}(\mathcal{G}_2)}\frac{1}{\omega(\mathcal{G}_2)} f(\mathcal{S}^{\star}\setminus \mathcal{A}^{\star}(\mathcal{S}^{\star}|\mathcal{G})) \label{ineq:thm1_na_ratio6}
\end{align}
where $k\in\{1,\cdots, \mathcal{K}(\mathcal{G}_2)\}$, $\gamma =\max[\frac{1}{\alpha+1}, \frac{1}{N-\alpha}] $ and 
\[
    h^{}_{k}=\left\{
                \begin{array}{ll}
                \frac{1}{n_{2,k}}, ~\text{ if}~n_{2,k}=1 ~\text{or}~\\ ~~~~~~~~\mathcal{C}_k(\mathcal{G}_2)~\text{has an oblivious decision}, \\
             \frac{1}{2}, ~~~~~\text{else}.
                \end{array}
              \right.
  \]
$\mathcal{S}_{2,k}^{}|\mathcal{C}_k(\mathcal{G}_2)$ is the strategy set of Algorithm~\ref{alg:DRA} on the clique $\mathcal{C}_k(\mathcal{G}_2)$ 
and $n_{2,k}$ is its carnality. Eqs.~\ref{ineq:thm1_na_ratio1}-\ref{ineq:thm1_na_ratio6} hold for the following reasons. Ineq.~\ref{ineq:thm1_na_ratio1} holds from~\cite[the proof of Theorem 1]{tzoumas2018resilient}. Ineq.~\ref{ineq:thm1_na_ratio2} holds from the monotonicity of the submodular function $f$: $f(\mathcal{S}_2^{}|\mathcal{G}_2) \geq f(\mathcal{S}_{2,k}^{}|\mathcal{C}_k(\mathcal{G}_2))$ for all $k\in \{1,\cdots, \mathcal{K}(\mathcal{G}_2)\}$. Ineq.~\ref{ineq:thm1_na_ratio3} holds from the distributed resilient algorithm (Alg.~\ref{alg:DRA}) in each clique. As long as the clique $\mathcal{C}_k(\mathcal{G}_2)$ has an oblivious strategy, $f(\mathcal{S}_{2,k}^{fd}|\mathcal{C}_k(\mathcal{G}_2)) \geq \frac{1}{n_{2,k}} f(\mathcal{S}_{2,k}^{\star}|\mathcal{C}(\mathcal{G}_2))$. That is because the oblivious approach picks the strategy with the largest contribution without the consideration of the redundancy. There is a special case where the \emph{local $\alpha$ largest set} of the clique $\mathcal{C}_k(\mathcal{G}_2)$ is exactly the \emph{central largest $\alpha$ set}. In this case, this clique $\mathcal{C}_k(\mathcal{G}_2)$ only performs a greedy algorithm. Because its oblivious strategy set are picked as the  \emph{central $\alpha$ largest set}. In this case, $f(\mathcal{S}_{2,k}^{}|\mathcal{C}_k(\mathcal{G}_2)) \geq \frac{1}{2} f(\mathcal{S}_{2,k}^{\star}|\mathcal{C}(\mathcal{G}_2))$ which is from the property of the greedy algorithm~\cite[Theorem 2.3]{conforti1984submodular} and $\mathcal{S}_{2,k}^{\star}|\mathcal{C}_k(\mathcal{G}_2)$ denotes the optimal strategy set on the clique $\mathcal{C}_k(\mathcal{G}_2)$.  Also, when $n_{2,k}=1$, both an oblivious strategy and a greedy strategy are the same as the optimal strategy and have 1 approximation. Ineq.~\ref{ineq:thm1_na_ratio4} holds obviously from ineq.~\ref{ineq:thm1_na_ratio3}. To explain ineq.~\ref{ineq:thm1_na_ratio5}, we compute 
$\min_{k} h^{}_{k}$ as
  \[
   \left\{
                \begin{array}{ll}              \frac{1}{\omega(\mathcal{G}_2)}, ~\text{if}~n_{2,k}=1~\text{for all}~k\in\{1,\cdots, \mathcal{K}(\mathcal{G}_2)\}\\
          ~~~~~~~~~~\text{or all}~ \mathcal{C}_k(\mathcal{G}_2)~k\in\{1,\cdots, \mathcal{K}(\mathcal{G}_2)\}\\~~~~~~~~~~\text{have at least an oblivious decision}, \\
             \min_k [\frac{1}{n_{2,k}}, \frac{1}{2}], \text{for all}~k\in\{1,\cdots, \mathcal{K}(\mathcal{G}_2)\}~  \\
             ~~~~~~~~~~~\text{except the one corresponds to the clique }\\ ~~~~~~~~~~~\text{that only has greedy strategies}, ~\text{else}.
                \end{array}
              \right.
  \]
Given $\omega(\mathcal{G}_2)$ is the clique number of the subgraph $\mathcal{G}_2$, we have $\omega(\mathcal{G}_2) \geq n_{2,k}$ for all $k$. If there exists one clique $\mathcal{C}_k(\mathcal{G}_2)$ containing more than one robot, $n_{2,k} \geq 2$. Thus, overall, $\min_{k} h^{}_{k} \geq \frac{1}{\omega(\mathcal{G}_2)}$, and therefore ineq.~\ref{ineq:thm1_na_ratio5} holds from the submodularity of the function $f$. Ineq.~\ref{ineq:thm1_na_ratio6} holds from ~\cite[Lemma 2]{orlin2018robust}. 

Combining the proofs of ineqs.~\ref{ineq:thm1_appx_ratio1}, \ref{ineq:thm1_appx_ratio2}, and~\ref{ineq:thm1_appx_ratio3}, we prove the approximation ratio in Theorem~\ref{thm:DRA}.

% \textbf{Number of communications}: The number of communications in Algorithm~\ref{alg:DRA} comes from both the distributed non-overlapping clique cover (Alg.~\ref{alg:DNCCA}) and the local resilient algorithm. In Algorithm~\ref{alg:DRA}, the robots talks with their neighbors in three rounds in parallel. We focus on the robot which has the largest number of neighbors. Thus, the number of communications for  Algorithm~\ref{alg:DRA} is $3\max_{i\in\mathcal{R}}[\mathcal{N}_i]$. 
% Then, by performing a local resilient algorithm, every two robots in a clique need to communicate. We focus on the clique of graph $\mathcal{G}$ which has the largest number of robots. Thus, the communication for the local resilient algorithm is $\binom{\omega(\mathcal{G})}{2}$. Overall, the number of communications for Algorithm~\ref{alg:DRA} is $3\max_{i\in\mathcal{R}}[\mathcal{N}_i] +  \binom{\omega(\mathcal{G})}{2}$.  
\textbf{Proof of running time.} 
% The running time of Algorithm~\ref{alg:DRA} also comes from two parts, Algorithm~\ref{alg:DNCCA} and the following local resilient algorithm. 
% In Algorithm~\ref{alg:DNCCA}, a robot needs to compute $\binom{\mathcal{N}^{+}}{m}$ combinations from $m= |\mathcal{\mathcal{N}}_i|+1$ to $m = 2$ in the worst-case for identifying all the maximal cliques (Alg.~\ref{alg:DNCCA}, lines~\ref{line:ncc_m_for_1}-\ref{line:ncc_m_for_end}).  Thus, in the worst-case scenario, the robots takes $O(2^{|\mathcal{N}_i|+1})$ evaluations for computing maximal cliques. Then, it takes  $O\binom{|\mathcal{N}_i|+1}{2} \log (O\binom{|\mathcal{N}_i|+1}{2})$ evaluations to rank out an unique maximal clique in the worst-case scenario, e.g., $m=2$ (Alg.~\ref{alg:DNCCA}, line~\ref{line:ncc_pick_one_unique}). Overall, Algorithm~\ref{alg:DNCCA} takes $O(2^{\max_{i\in\mathcal{R}}[\mathcal{N}_i]+1})$ time by evaluating the robot with largest number of neighbors.  
Next, since all cliques perform a local resilient  algorithm in parallel, we only focus on the clique which has the largest number of the robots. We know the number of the robots in this clique is the clique number of the graph, $\omega(\mathcal{G})$. Given each robot has $D$ candidate decisions, the oblivious approach takes $ O(\omega(\mathcal{G})D\log(\omega(\mathcal{G})D))$ evaluations to rank out the \emph{local $\alpha$ largest set} by using \emph{quick sort}. And then the greedy approach takes $O((\omega(\mathcal{G})-\alpha)^2D^2)$ evaluations for the remaining robots if $\omega(\mathcal{G})> \alpha$. If $\omega(\mathcal{G}) \leq \alpha$, the greedy algorithm has nothing to do, and thus takes $0$ evaluations.  Thus, overall, algorithm~\ref{alg:DRA} takes $O(\omega^2(\mathcal{G})D^2)$ time.
